# Supplementary material for: Quantitative Imaging Principles Improves Medical Image Learning
Source: arXiv:2206.06663 source file (2022-07-11)
Supplement: Supplementary file 1 [file appendix.tex]

\appendix
\section{Modeling Details}
\label{app:modeling}
All modeling and experiments were implemented in Tensorflow and Keras and performed on a NVIDIA DGX-1 64-bit Linux system with 1TB of RAM and NVIDIA tesla v100 GPUs. DXA images were kept in their native resolution 150 $\times$ 109 $\times$ 6 (height, width, channel) and normalized between [0, 1]. A subset of the same 22K vertices from the 100K standardized 3D body  meshes were used for modeling and experiments. Hyperparameters were optimized for all models using SHERPA~\cite{sherpa} and were kept consistent for each experiment, see Table~\ref{tab:params}. Code is at~\url{https://github.com/LambertLeong/DXA-VAE}.

\iffalse
\begin{table}[]
\begin{tabular}{lrrr}
Hyperparameter & \multicolumn{1}{l}{SSL DXA-VAE} & \multicolumn{1}{l}{\begin{tabular}[c]{@{}l@{}}DXA-VAE \\ Encoder \\ Experiements\end{tabular}} & \multicolumn{1}{l}{\begin{tabular}[c]{@{}l@{}}DXA-VAE \\ Generator \\ Experiements\end{tabular}} \\
Data Input & DXA Scan & DXA Scan & 3D Bod Scan Mesh \\
Data Output & DXA Scan & 3D Anthropometry & DXA Scan \\
Learning Rate & 1.00E-07 & 0.0003 & 5.00E-07 \\
Beta & 0.5 & 0.2 & 0.3 \\
Dropout & 0 & 0.14 & 0.09 \\
Optimizer & Adam & Adam & Adam \\
Batch Size & 32 & 32 & 8 \\
Epochs & 122 & 83 & 69
\end{tabular}
\end{table}
\fi

\begin{table}[h!]
  \caption{Hyperparameters used for all models and experiments.}
  \label{tab:params}
  \centering
\resizebox{.8\textwidth}{!}{
\begin{tabular}{lrrr}
\toprule
Hyperparameter & \multicolumn{1}{l}{SSL DXA-VAE} & \multicolumn{1}{l}{\begin{tabular}[c]{@{}l@{}}DXA-VAE \\ Encoder \\ Experiements\end{tabular}} & \multicolumn{1}{l}{\begin{tabular}[c]{@{}l@{}}DXA-VAE \\ Generator \\ Experiements\end{tabular}} \\
\midrule
\midrule
Data Input & DXA Scan & DXA Scan & 3D Bod Scan Mesh \\
Data Output & DXA Scan & 3D Anthropometry & DXA Scan \\
Learning Rate & 1.00E-07 & 0.0003 & 5.00E-07 \\
Beta & 0.5 & 0.2 & 0.3 \\
Dropout & 0 & 0.14 & 0.09 \\
Optimizer & Adam & Adam & Adam \\
Batch Size & 32 & 32 & 8 \\
Epochs & 122 & 83 & 69 \\
\bottomrule
\end{tabular}
}
\end{table}

%\section{Measuring Body Composition}

\clearpage
